# Supplementary material for: Stochastic and Mixed Density Functional Theory within the projector augmented wave formalism for the simulation of warm dense matter
Source: arXiv:2301.12018 source file (2023-01-27)
Supplement: Supplementary file 1 [file PAW_sDFT_SI.pdf]

**Supplementary Information for**

# Stochastic and Mixed Kohn Sham Density Functional theory within the projector augmented wave formalism for simulation of warm dense matter

Vidushi Sharma[1,2], Lee A. Collins[1], and Alexander J. White[1]
[1] *Theoretical Division, Los Alamos National Laboratory, Los Alamos, NM 87545, USA*
[2] *Center for Nonlinear Studies (CNLS), Los Alamos National Laboratory, Los Alamos, NM 87545, USA*
(Dated: January 27, 2023)

## S1. BASIC PAW TRANSFORMATION IDENTITIES

Here we review some useful definitions and identities for deriving PAW transformations. Particularly, transformations of orbitals, stochastic vectors and operators, a useful resolution of the identity, and arbitrary functions of operators.

The Basic PAW transformation operator, $\widehat{\tau}$, is defined by:

$$|\Psi\rangle = |\tilde{\Psi}\rangle + \sum_i \big(|\phi_i\rangle - |\tilde{\phi}_i\rangle\big)\langle p_i|\tilde{\Psi}\rangle \equiv \widehat{\tau}|\tilde{\Psi}\rangle \ , \tag{S1}$$

$$\langle\Psi| = \langle\tilde{\Psi}|\widehat{\tau}^\dagger \ , \tag{S2}$$

where $|\Psi\rangle$ is a vector representing the electronic state, *i.e.*, a KS-orbital or stochastic vector. The projectors ($|p_i\rangle$) and smooth partial-waves ($|\tilde{\phi}_i\rangle$) form a biorthogonal dual space :

$$\delta_{i,j} = \langle p_i|\tilde{\phi}_j\rangle \ , \tag{S3}$$

$$\widehat{I} = \sum_i |\tilde{\phi}_i\rangle\langle p_i| \ . \tag{S4}$$

The transformation of an all-electron operator (exact only for a complete basis of projectors and partial waves) is defined so as to conserve the expectation value. Here for simplicity we assume $|\Psi\rangle$ are eigenstates of the KS Hamiltonian:

$$\langle\widehat{O}\rangle = \sum_i \langle\Psi_i|\widehat{O}|\Psi_i\rangle f(\varepsilon_i) \equiv \sum_i \langle\tilde{\Psi}_i|\widetilde{O}|\tilde{\Psi}_i\rangle f(\varepsilon_i) \tag{S5}$$

$$\begin{aligned}\widetilde{O} &\equiv \widehat{\tau}^\dagger\widehat{O}\widehat{\tau} = \widehat{O} + \sum_{i,j}|p_i\rangle(\langle\phi_i|\widehat{O}|\phi_j\rangle - \langle\tilde{\phi}_i|\widehat{O}|\tilde{\phi}_j\rangle)\langle p_j| \\ &= \widehat{O} + \sum_{i,j}|p_i\rangle o_{ij}\langle p_j| \ .\end{aligned} \tag{S6}$$

As a critical example, the transformation of the identity operator leads to the S-orthogonality condition for PAW transformed KS-orbitals:

$$\begin{aligned}\widehat{S} &\equiv \widetilde{I} \equiv \widehat{\tau}^\dagger\widehat{\tau} \\ &= \widehat{I} + \sum_{i,j}|p_i\rangle(\langle\phi_i|\phi_j\rangle - \langle\widetilde{\phi}_i|\tilde{\phi}_j\rangle)\langle p_j| = \widehat{I} + \sum_{i,j}|p_i\rangle s_{ij}\langle p_j| \\ \langle\Psi_a|\Psi_b\rangle &= \langle\tilde{\Psi}_a|\widehat{S}|\tilde{\Psi}_b\rangle = \delta_{a,b} \ .\end{aligned} \tag{S7}$$

A useful resolution of the identity helps to relate the transformed product of operators to the transformed operators. It is defined by:

$$\begin{aligned}\widehat{I} &= \tau\widehat{S}^{-1}\tau^\dagger \ \text{, where} \\ \widehat{S} &= \widehat{\tau}^\dagger\widehat{\tau} = \widehat{S}\widehat{S}^{-1}\widehat{S} = \widehat{\tau}^\dagger\widehat{\tau}\widehat{S}^{-1}\tau^\dagger\widehat{\tau} = \widehat{\tau}^\dagger\widehat{I}\widehat{\tau} \ .\end{aligned} \tag{S8}$$

The transformation of products and (analytic) functions of operators is then easily obtained:

$$\begin{aligned}\widehat{\tau}^\dagger \widehat{A}\widehat{B}\widehat{\tau} &= \widehat{\tau}^\dagger \widehat{A}\tau\widehat{S}^{-1}\tau^\dagger\widehat{B}\widehat{\tau} \\ &= \widetilde{A}\widehat{S}^{-1}\widetilde{B}\ , \end{aligned} \tag{S9}$$

$$\begin{aligned}\widehat{\tau}^\dagger f(\widehat{A})\widehat{\tau} &= \sum_\gamma^\infty c_\gamma(f)\ \widehat{\tau}^\dagger \widehat{A}^\gamma\widehat{\tau} = \sum_\gamma^\infty c_\gamma(f)\widehat{S}(\widehat{S}^{-1}\widetilde{A})^\gamma \\ &= \widehat{S}\ f(\widehat{S}^{-1}\widetilde{A})\ , \end{aligned} \tag{S10}$$

where $c_\gamma(f)$ is the $\gamma^{th}$ polynomial expansion coefficient for the function $f$.

The KS density matrix is then given as:

$$\rho(\widehat{H}) = \sum_i \widehat{\tau} f^{1/2}(\widehat{S}^{-1}\widetilde{H})|\tilde{\Psi}_i\rangle\langle\tilde{\Psi}_i|f^{1/2}(\widetilde{H}\widehat{S}^{-1})\widehat{\tau}^\dagger \equiv \widehat{\tau}\widetilde{\rho}(\widetilde{H})\widehat{\tau}^\dagger\ , \tag{S11}$$

which allows for expectation values to be calculated as:

$$E[\widehat{O}] = \mathrm{Tr}[\widehat{\rho}\,\widehat{O}] = \mathrm{Tr}[\widetilde{\rho}\,\widetilde{O}]\ . \tag{S12}$$

To avoid potential confusion, we note that one could define the transformed KS density matrix such that it follows the convention of operators:

$$\widetilde{\rho}\,'(\widetilde{H}) \equiv \widehat{\tau}^\dagger\rho(\widehat{H})\widehat{\tau} = \widehat{S}f(\widehat{S}^{-1}\widetilde{H}) = \widehat{S}\widetilde{\rho}(\widetilde{H})\widehat{S}\,, \tag{S13}$$

but then the expectation values have the less concise form:

$$E[\widehat{O}] = \mathrm{Tr}[\widehat{\rho}\,\widehat{O}] = \mathrm{Tr}[\widetilde{\rho}\,'\widehat{S}^{-1}\,\widetilde{O}\widehat{S}^{-1}] = \mathrm{Tr}[f(\widehat{S}^{-1}\widetilde{H})\,\widehat{S}^{-1}\,\widetilde{O}] = \mathrm{Tr}[\widetilde{\rho}\,\widetilde{O}]\ . \tag{S14}$$

## S2. PAW TRANSFORMATION FOR HELLMANN FEYNMAN FORCE AND STRESS TENSOR

The all-electron force obeys the Hellman-Feynman theorem. As such it is the starting point for the forces within the PAW formalism.

$$\vec{F}_{at} = -\mathrm{Tr}[\frac{\partial}{\partial\vec{R}_{at}}\widehat{H}\,\widehat{\rho}] = -\mathrm{Tr}[\,\widehat{\tau}^\dagger\frac{\partial}{\partial\vec{R}_{at}}\widehat{H}\widehat{\tau}\,\widetilde{\rho}]\ . \tag{S15}$$

Special care must be taken when dealing with derivatives with respect to the atom positions, as the PAW projectors are centered at the atom positions. Using the resolution of identity, Eq. (S8):

$$\begin{aligned}\widehat{\tau}^\dagger\frac{\partial}{\partial\vec{R}_{at}}\widehat{H}\widehat{\tau} &= \widehat{\tau}^\dagger\left[\frac{\partial}{\partial\vec{R}_{at}}\widehat{\tau}\widehat{S}^{-1}\widetilde{H}\widehat{S}^{-1}\widehat{\tau}^\dagger\right]\widehat{\tau} \\ \widehat{\tau}^\dagger\frac{\partial}{\partial\vec{R}_{at}}\widehat{\tau} &= \widehat{D} + \widehat{S}\frac{\partial}{\partial\vec{R}_{at}} \\ \widehat{D} &\equiv -\sum_{i,j}|p_i\rangle\vec{\nabla}_{ij}\langle p_j| + \sum_{i,j}|p_i\rangle s_{ij}\langle\frac{\partial p_j}{\partial\vec{R}_{at}}| \\ \frac{\partial}{\partial\vec{R}_{at}}\widehat{S}^{-1} &= -\widehat{S}^{-1}\left[\frac{\partial}{\partial\vec{R}_{at}}\widehat{S}\right]\widehat{S}^{-1} = -\widehat{S}^{-1}\left[D+D^\dagger\right]\widehat{S}^{-1}\ ,\end{aligned} \tag{S16}$$

where $\vec{\nabla}_{ij}$ is the on-site gradient matrix, and $s_{ij}$ is the on-site overlap matrix. Applying the chain rule and doing some algebra:

$$\vec{F}_{at} = -\,\mathrm{Tr}\left[\frac{\partial}{\partial\vec{R}_{at}}\widetilde{H}_{KS}\,\widetilde{\rho}\right] + 2\Re\{\mathrm{Tr}\left[(\,\widehat{D} - \frac{\partial}{\partial\vec{R}_{at}}\widehat{S}\,)\widehat{S}^{-1}\widetilde{H}_{KS}\,\widetilde{\rho}\right]\} \tag{S17}$$

$$= -\sum_a\langle\tilde{\Psi}_a|\frac{\partial}{\partial\vec{R}_{at}}\widetilde{H}_{KS} - \varepsilon_a\left[\frac{\partial}{\partial\vec{R}_{at}}\widehat{S}\right]|\tilde{\Psi}_a\rangle f(\varepsilon_a)\ . \tag{S18}$$

Eq. (S17) is valid for any representation of the density matrix, while Eq. (S18) assumes that $|\Psi\rangle$ is an eigenstate of $\widehat{H}$. The derivative of the transformed KS Hamiltonian and $\widehat{S}$ can be found in standard PAW references [1, 2].

Similarly, for stress tensor ($W_{x,y}$), we have:

$$W_{x,y} = \frac{1}{\Omega}\left\{\mathrm{Tr}\left[\frac{\partial}{\partial\epsilon_{x,y}}\widetilde{H}\,\widetilde{\rho}\right] + 2\Re\left\{\mathrm{Tr}\left[(\widehat{G}_{xy} - \frac{\partial}{\partial\epsilon_{x,y}}\widehat{S})\widehat{S}^{-1}\widetilde{H}\,\widetilde{\rho}\right]\right\}\right\} \tag{S19}$$

$$= \frac{1}{\Omega}\sum_a \langle\tilde{\Psi}_a|\frac{\partial}{\partial\epsilon_{x,y}}\widetilde{H} - \varepsilon_a\left[\frac{\partial}{\partial\epsilon_{x,y}}\widehat{S}\right]|\tilde{\Psi}_a\rangle f(\varepsilon_a)\ . \tag{S20}$$

Again the first expression is valid for any $\widetilde{\rho}$ representation, while the second assumes $|\Psi\rangle$ is an eigenstate of $\widehat{H}$. The derivative of the pseudized Hamiltonian can be found in Refs. [1, 2]. The explicit term involving the derivative with respect to the pseudized identity operator ($\widehat{S}$) is calculated as:

$$\widehat{G}_{xy} = \delta_{x,y}\widehat{S} + \sum_{at,i,j}|p_i\rangle[y\nabla_x]_{ij}\langle p_j| - \sum_{at,i,j}|p_i\rangle s_{i,j}\langle\frac{\partial p_j}{\partial R_{at,y}}|(\widehat{r}_y - R_{at,x})\ , \tag{S21}$$

and

$$\frac{\partial}{\partial\epsilon_{x,y}}\widehat{S} = \delta_{x,y}\widehat{S} - \sum_{at,i,j}(\widehat{r}_y - R_{at,y})|\frac{\partial p_i}{\partial R_{at,x}}\rangle s_{at,ij}\langle p_j| - \sum_{at,i,j}|p_i\rangle s_{i,j}\langle\frac{\partial p_j}{\partial R_{at,y}}|(\widehat{r}_y - R_{at,x})\ . \tag{S22}$$

We have added the on-site stress matrix elements $[y\nabla_x]_{ij}$ to our local version of the `LibPAW` library leveraging the existing routines for calculating $\nabla_{ij}$.

## S3. MIXED AND STOCHASTIC DFT: ENERGIES, PRESSURES AND SCF TIMES

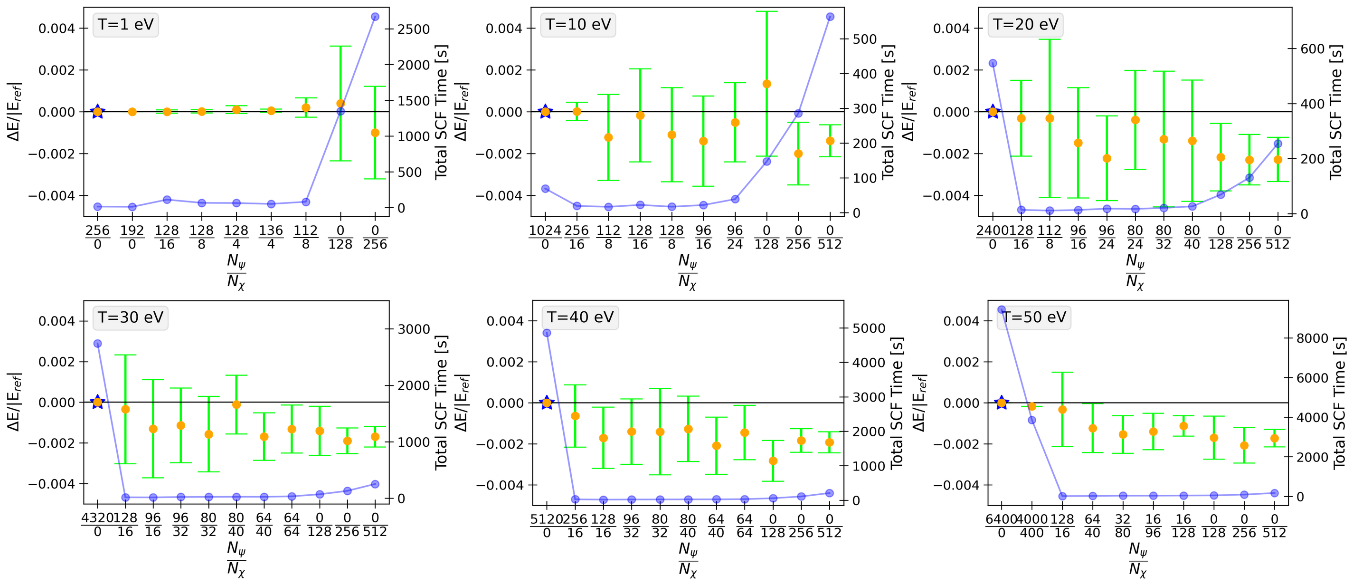


FIG. S1: Comparison of relative error in free energy and time taken for an SCF cycle convergence for different $N_\psi/N_\chi$ combinations. An optimal $N_\psi/N_\chi$ is chosen such that the bias is low and the reference energy is contained within the error margins, along with obtaining a good speedup in the SCF convergence.

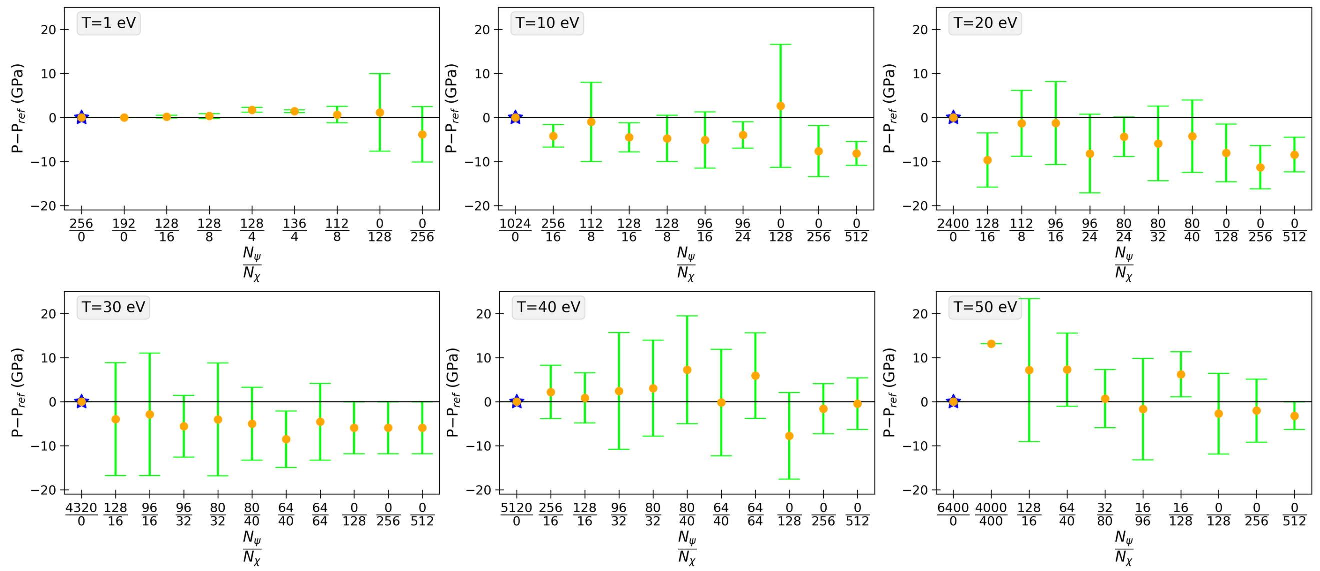


FIG. S2: Comparison of pressure with respect to the deterministic KS pressure ($P_{ref}$) for different $N_\psi/N_\chi$ combinations.

Figure S1 shows the relative error in free energies with respect to the reference energies ($E_{ref}$) from deterministic KS-DFT, along with the SCF times for a convergence cycle. The horizontal axis spans fully deterministic KS-DFT $N_\psi$'s on the left to purely stochastic DFT $N_\chi$'s on the right, with the mixed DFT $N_\psi/N_\chi$'s in the middle. The switch in relative computational time between KS-DFT and sDFT is seen as expected, as the temperature increases ($\sim 20$ eV). Mixed DFT remains more robust between the deterministic and stochastic ends across temperatures; and affords several choices in $N_\psi/N_\chi$ with reasonable SCF times and accuracy.

The difference in pressures computed in reference to the deterministic KS pressures ($P_{ref}$) is shown in Fig. S2. In mDFT and sDFT, the energies and pressures are computed as averages over ten independent runs, and the error bar

is taken to be the standard deviation of the mean. The reference values computed with KS-DFT are listed in Table S1, along with the values computed with mixed and stochastic DFT. Figure S3 shows a comparison of the three DFT algorithms in terms of computational speedup on 128 CPU cores, and the accuracy and precision of observables such as free energy, pressure, and chemical potential with varying temperatures. The free energy represented in Fig. S3(b) and Table S1 comprises Hartree, kinetic, exchange-correlation, core-electron, local ion, PAW on-site, nuclear potential and entropy, components of energy. The combination of orbitals $N_\psi/N_\chi$ ($N_\psi$) used for determining SCF times in mixed (Kohn Sham) DFT are listed in Table S1, whereas sDFT times are computed with $N_\chi = 128$ orbitals for all temperatures.

TABLE S1: Disordered carbon at $\rho = 3.52$ g/cc with a $4e^-$ PAW potential. $E_{\psi\chi}$ ($E_\psi$, $E_\chi$), $\mu_{\psi\chi}$ ($\mu_\psi$, $\mu_\chi$), and $P_{\psi\chi}$ ($P_\psi$, $P_\chi$) indicate the free energy per atom, chemical potential, and pressure computed using a mixed (Kohn Sham, stochastic) DFT approach. All stochastic values are reported for $N_\chi = 128$.

| T [eV] | mixed DFT | | | | KS-DFT | | | | sDFT | | |
|---|---|---|---|---|---|---|---|---|---|---|---|
| | $N_\psi/N_\chi$ | $E_{\psi\chi}$ [eV] | $\mu_{\psi\chi}$ [eV] | $P_{\psi\chi}$/1E2 [GPa] | $N_\psi$ | $E_\psi$ [eV] | $\mu_\psi$ [eV] | $P_\psi$/1E2 [GPa] | $E_\chi$ [eV] | $\mu_\chi$ [eV] | $P_\chi$/1E2 [GPa] |
| 1 | 136/4 | $-152.49 \pm 0.01$ | $11.04 \pm 0.03$ | $1.73 \pm 0.01$ | 256 | $-152.50$ | 10.97 | 1.72 | $-152.44 \pm 0.42$ | $11.08 \pm 0.15$ | $1.73 \pm 0.09$ |
| 3 | 136/4 | $-155.71 \pm 0.08$ | $10.83 \pm 0.09$ | $2.92 \pm 0.02$ | 512 | $-155.68$ | 10.75 | 2.94 | $-155.62 \pm 0.36$ | $10.88 \pm 0.10$ | $2.92 \pm 0.08$ |
| 5 | 128/8 | $-161.50 \pm 0.17$ | $10.53 \pm 0.12$ | $4.46 \pm 0.02$ | 768 | $-161.47$ | 10.41 | 4.48 | $-161.77 \pm 0.45$ | $10.43 \pm 0.13$ | $4.41 \pm 0.08$ |
| 10 | 128/16 | $-185.41 \pm 0.41$ | $7.98 \pm 0.18$ | $9.12 \pm 0.03$ | 1024 | $-185.37$ | 7.86 | 9.17 | $-185.12 \pm 0.64$ | $8.03 \pm 0.16$ | $9.19 \pm 0.14$ |
| 15 | 128/16 | $-220.00 \pm 0.48$ | $3.10 \pm 0.17$ | $14.46 \pm 0.04$ | 1760 | $-219.83$ | 3.01 | 14.49 | $-220.30 \pm 0.36$ | $3.04 \pm 0.10$ | $14.39 \pm 0.05$ |
| 20 | 96/16 | $-262.74 \pm 0.69$ | $-3.58 \pm 0.20$ | $20.18 \pm 0.09$ | 2400 | $-262.35$ | $-3.65$ | 20.20 | $-262.92 \pm 0.42$ | $-3.66 \pm 0.13$ | $20.11 \pm 0.07$ |
| 30 | 96/32 | $-366.26 \pm 0.67$ | $-21.10 \pm 0.19$ | $32.31 \pm 0.07$ | 4320 | $-365.85$ | $-21.15$ | 32.36 | $-366.36 \pm 0.44$ | $-21.14 \pm 0.11$ | $32.30 \pm 0.06$ |
| 40 | 80/32 | $-488.75 \pm 1.03$ | $-42.89 \pm 0.29$ | $45.07 \pm 0.01$ | 5120 | $-488.07$ | $-42.93$ | 45.03 | $-489.45 \pm 0.48$ | $-43.10 \pm 0.12$ | $44.96 \pm 0.10$ |
| 50 | 64/40 | $-625.56 \pm 0.74$ | $-68.05 \pm 0.20$ | $58.11 \pm 0.08$ | 6400 | $-624.79$ | $-68.05$ | 58.04 | $-625.85 \pm 0.65$ | $-68.14 \pm 0.14$ | $58.01 \pm 0.09$ |

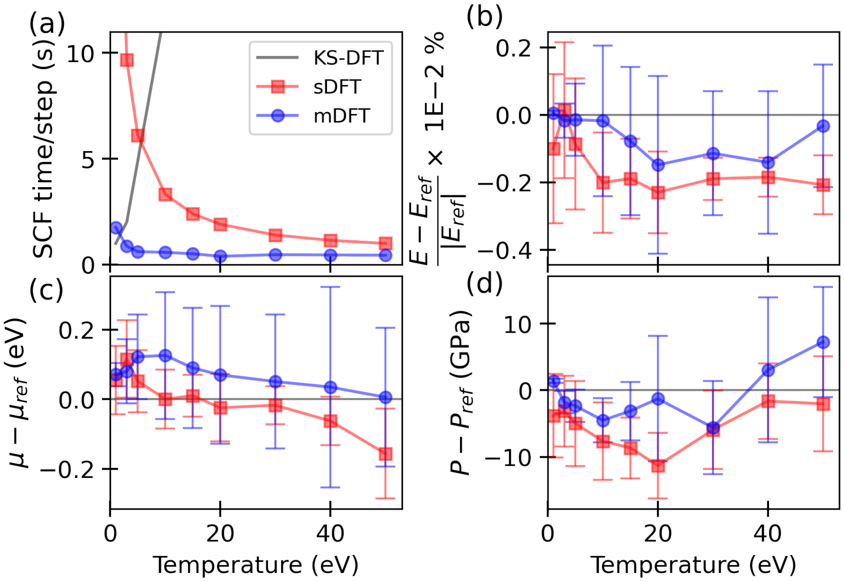


FIG. S3: Carbon disordered system comprising 64 atoms at $\rho = 3.52$ g/cc. (a) SCF times per cycle compared for deterministic (Kohn Sham), stochastic, and mixed DFT calculations performed using a cray compilation of SHRED on 128 cores. Comparison of (b) relative error in free energy, (c) chemical potential and, (d) pressure with reference to Kohn Sham DFT calculation shown in grey as a guide.

## S4. FORCES FROM STOCHASTIC AND MIXED KOHN SHAM DFT WITH PAW

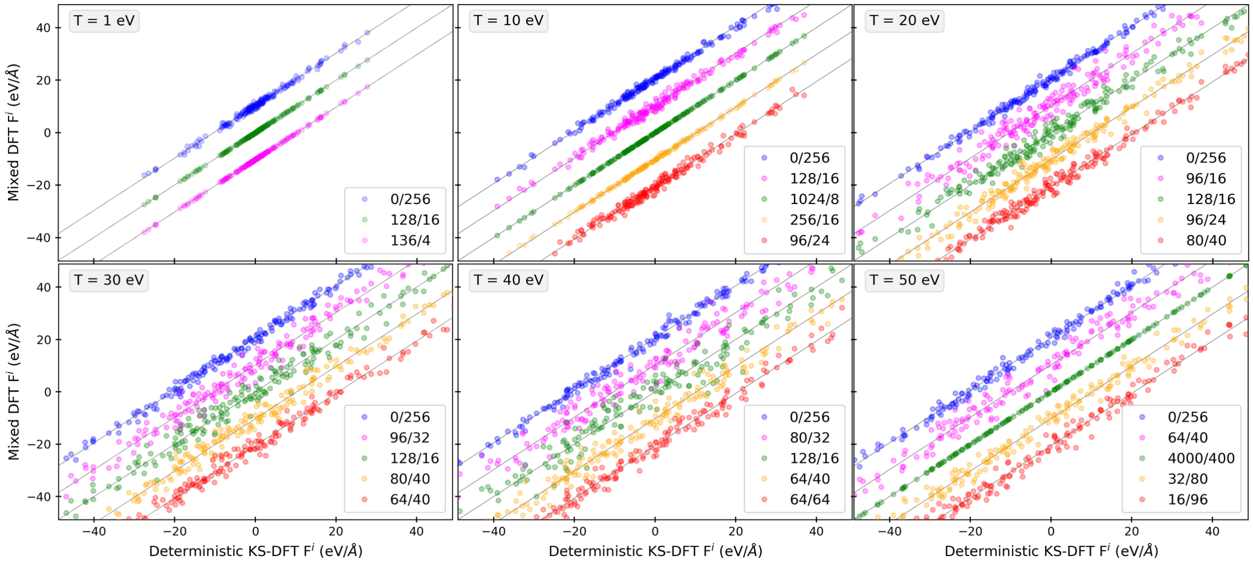


FIG. S4: Comparison of mixed DFT forces obtained for a $N_\psi/N_\chi$ vs. deterministic Kohn Sham forces at a given temperature T.

All components of forces, $\mathrm{F}^i_\alpha$, are shown as a comparison between mixed/stochastic and KS-DFT in Fig. S4, and the average magnitude of force on the atoms along with the standard deviation in the forces from mixed runs is presented in Table S2. For mixed DFT, several $N_\psi/N_\chi$ combinations are sampled at each T.

TABLE S2: Forces for a single snapshot of disordered carbon at $\rho = 3.52$ g/cc with a $4e^-$ PAW potential. $\mathrm{F}^{\psi\chi}$ and $\sigma^{\psi\chi}$ indicate the mean of atomic force magnitudes and standard deviation in the force magnitudes averaged over the atoms respectively obtained with mixed DFT ($N_\psi/N_\chi$). $\mathrm{F}^\psi$ is the deterministic Kohn Sham mean force given here for comparison.

| T [eV] | mixed DFT | | | KS-DFT | |
|---|---|---|---|---|---|
| | $N_\psi/N_\chi$ | $\mathrm{F}^{\psi\chi}$ [eV/Å] | $\sigma^{\psi\chi}$ [eV/Å] | $N_\psi$ | $\mathrm{F}^\psi$ [eV/Å] |
| 1 | 136/4 | 11.743 | 0.314 | 256 | 11.709 |
| 3 | 136/4 | 11.949 | 1.519 | 512 | 12.003 |
| 5 | 128/8 | 13.574 | 2.369 | 768 | 13.741 |
| 10 | 128/16 | 19.968 | 3.643 | 1024 | 20.371 |
| 15 | 128/16 | 26.466 | 5.850 | 1760 | 26.661 |
| 20 | 96/16 | 32.383 | 8.856 | 2400 | 32.202 |
| 30 | 96/32 | 42.027 | 8.647 | 4320 | 41.682 |
| 40 | 80/32 | 48.380 | 10.471 | 5120 | 49.660 |
| 50 | 64/40 | 56.622 | 10.364 | 6400 | 56.562 |

## S5. STOCHASTIC AND MIXED KOHN SHAM DFT FORCES IN THE PRESENCE OF LANGEVIN-FRICTION TERM

In Fig. S5, the blue-shaded band indicates thermal fluctuations due to the friction term, $\varsigma = \sqrt{2m_\alpha\gamma_\alpha k_B T}$, where $m_\alpha = 12$ a.u. is the atomic mass of carbon atom, and $\gamma_\alpha = 0.04$ fs$^{-1}$ is the damping constant. $\varsigma$ controls the temperature in Langevin dynamics in order to approximate a canonical ensemble:

$$m_\alpha \ddot{q}_\alpha = f_\alpha - \gamma_\alpha p_\alpha + \underbrace{\sqrt{2m_\alpha\gamma_\alpha k_B T}}_{\varsigma}\,\eta_\alpha(t)\ ,$$

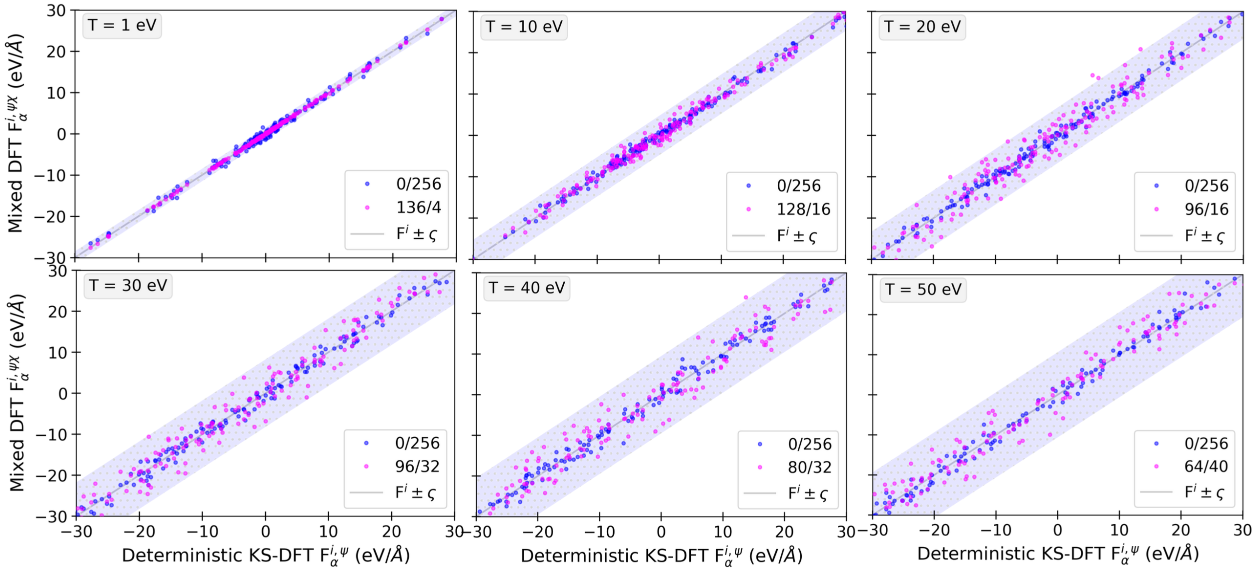


FIG. S5: Mixed DFT vs. Kohn Sham forces shown against a background of Langevin friction term ($\sigma$) computed at a given temperature. The mixed and stochastic force components ($F_\alpha^{i,\psi\chi}$) were averaged over ten independent runs on a single snapshot geometry of carbon atoms at $\rho = 3.52$ g/cc.

where $(q_\alpha, p_\alpha)$ are the coordinates and momenta of the atoms, $f_\alpha$ is the force on the atom, $k_B$ is the Boltzmann constant and $\eta_\alpha(t)$ is a Gaussian distribution function such that $\langle\eta_\alpha(t)\rangle = 0$ and $\langle\eta_\alpha(t)\eta_{\alpha'}(t')\rangle = \delta_{\alpha\alpha'}\delta(t-t')$. Figure S5 shows that the noise in stochastic forces could be absorbed by the thermal friction term at any given temperature, indicating an accurate molecular dynamics scenario.

## S6. MOLECULAR DYNAMICS: ENERGIES AND PRESSURES

Figure S6 shows the total free energy consisting of the electronic energy (Hartree, kinetic, exchange-correlation, core electron, local ion, PAW on-site) and nuclear potential while the system is coupled to an isokinetic thermostat. In addition to the mDFT MD runs, a deterministic KS-DFT MD run is presented for comparison at lower temperatures, and a purely sDFT MD run is shown at higher temperatures. The effect of increasing the stochastic orbitals ($N_\chi$) in mDFT MD is shown for the case of T=10 eV in going from $N_\psi/N_\chi$ : 128/16 (green) $\rightarrow$ 128/32 (grey) $\rightarrow$ 128/64 (cyan) in Fig. S6; where the energies tend toward the deterministic value at greater $N_\chi$.

The total pressure comprising Hartree, kinetic, exchange-correlation, core, local ion, non-local ion, core exchange-correlation, compensation charge due to PAW, nuclear kinetic and nuclear potential pressures is shown in Fig. S7. The time-averaged free energy per atom and pressure together with their standard deviations, are listed in Table S3 for the MD trajectories shown in Figs. S6, S7.

TABLE S3: Molecular dynamics for a disordered carbon system at $\rho = 3.52$ g/cc with a $4e^-$ PAW potential. $E_{\psi\chi}$ ($E_\psi$, $E_\chi$) and $P_{\psi\chi}$ ($P_\psi$, $P_\chi$) indicate the total free energy per atom and pressure computed using a mixed (Kohn Sham, stochastic) DFT approach. $\pm$ indicates the standard deviation over the trajectory.

| T [eV] | mixed DFT | | | KS-DFT | | | stochastic-DFT | | |
|---|---|---|---|---|---|---|---|---|---|
| | $N_\psi/N_\chi$ | $E_{\psi\chi}$ [eV] | $P_{\psi\chi}$/1E2 [GPa] | $N_\psi$ | $E_\psi$ [eV] | $P_\psi$/1E2 [GPa] | $N_\chi$ | $E_\chi$ [eV] | $P_\chi$/1E2 [GPa] |
| 1 | 136/4 | $-153.57 \pm 0.12$ | $16.40 \pm 0.18$ | 256 | $-153.59 \pm 0.13$ | $16.40 \pm 0.17$ | – | – | – |
| 5 | 128/8 | $-160.70 \pm 0.36$ | $18.59 \pm 0.37$ | 768 | $-161.22 \pm 0.34$ | $18.72 \pm 0.37$ | 128 | $-160.97 \pm 0.53$ | $18.64 \pm 0.39$ |
| 10 | 128/64 | $-184.10 \pm 0.69$ | $23.09 \pm 0.43$ | 1024 | $-184.21 \pm 0.66$ | $23.19 \pm 0.41$ | 256 | $-184.25 \pm 0.71$ | $23.11 \pm 0.47$ |
| 20 | 96/64 | $-258.84 \pm 1.35$ | $33.90 \pm 0.46$ | – | – | – | 256 | $-259.48 \pm 1.30$ | $33.90 \pm 0.49$ |
| 30 | 96/32 | $-358.61 \pm 1.97$ | $45.83 \pm 0.51$ | – | – | – | 256 | $-361.06 \pm 1.86$ | $45.90 \pm 0.51$ |
| 40 | 80/32 | $-477.81 \pm 2.49$ | $58.52 \pm 0.52$ | – | – | – | 256 | $-481.52 \pm 2.45$ | $58.56 \pm 0.52$ |
| 50 | 64/40 | $-612.54 \pm 2.91$ | $71.43 \pm 0.54$ | – | – | – | 256 | $-616.20 \pm 2.90$ | $71.40 \pm 0.54$ |

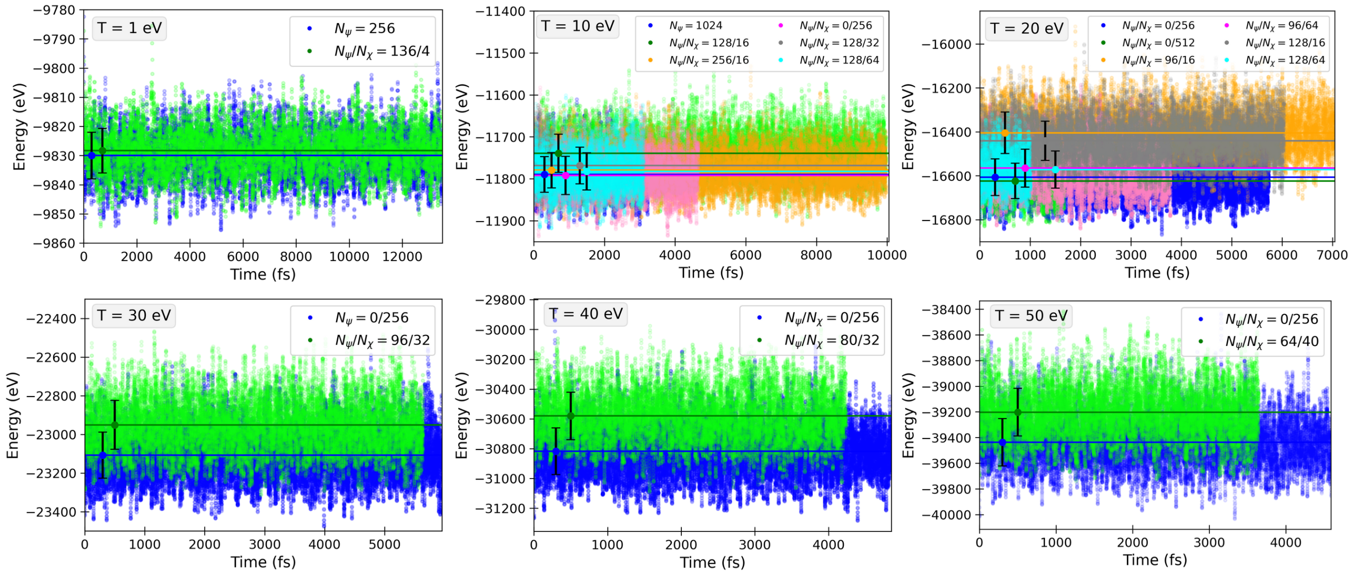


FIG. S6: Total free energy during an isokinetic thermostatted molecular dynamics run using KS-DFT ($N_\psi$), mDFT ($N_\psi/N_\chi$), and sDFT ($N_\chi$). The mean and standard deviation of the free energy computed over time is also shown.

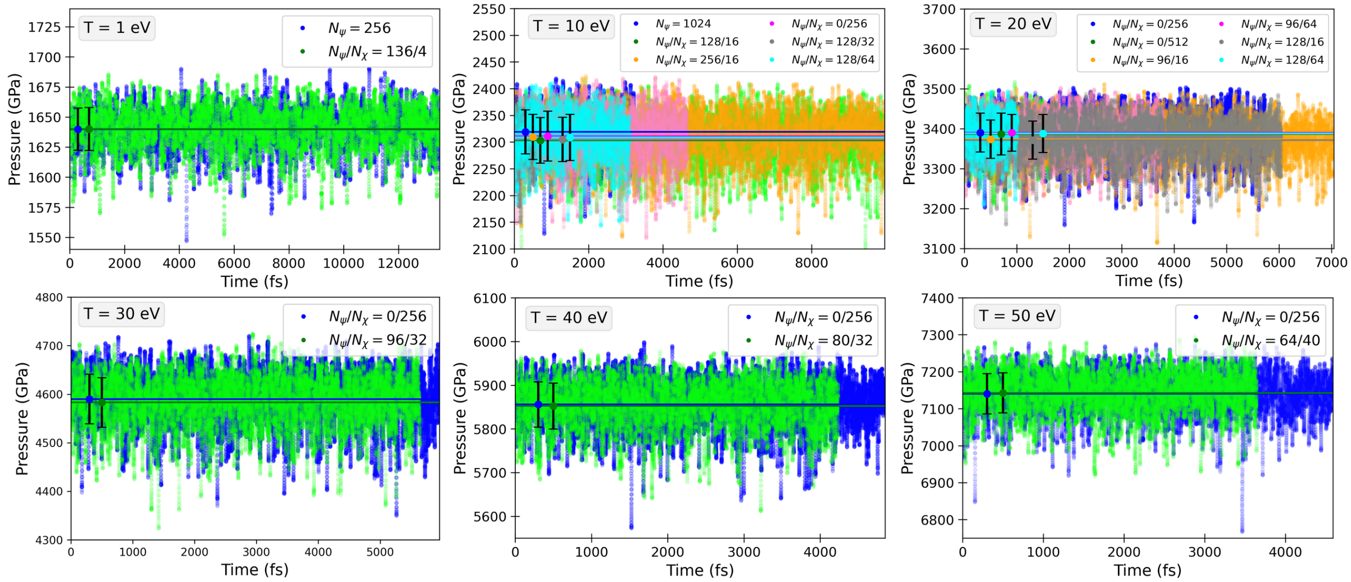


FIG. S7: Total electronic and nuclear pressure during an isokinetic thermostatted molecular dynamics run using KS-DFT ($N_\psi$), mDFT ($N_\psi/N_\chi$), and sDFT ($N_\chi$). The mean and standard deviation of the pressure computed over time is also shown as solid dots and horizontal lines with error bars.

## S7. STATISTICAL ERROR ESTIMATION IN SELF-DIFFUSION COEFFICIENT

Velocity autocorrelation functions and self-diffusions (D)are calculated from the ion velocities ($v_a$) as

$$\vec{V}(t) = \frac{1}{N_a} \sum_a \vec{v}_a(t) \; , \tag{S23}$$

$$\mathrm{VACF}(t) = \frac{dt}{3N_{t_0}} \sum_{t_0} \vec{V}(t_0) \cdot \vec{V}(t_0 + t) \; , \tag{S24}$$

$$D = dt \sum_t \mathrm{VACF}(t) \; , \tag{S25}$$

where the sum over $t_0$ includes every timestep except for an initial equilibration time. Thus the average VACFs include $N_{t_0}$ overlapping individual VACFs. This overlap must be accounted for when estimating the error in the VACF/Diffusion coefficient. For calculating the standard error from the standard deviation, one needs to divide by the square root of the number of independent samples. Taking $t_0$ at every time point leads to a smoother VACF by averaging over some high frequency noise, but the samples are not fully independent. Thus one needs to estimate the number of independent samples by estimating a decorrelation time, $t_D$.

$$St.Error = St.Dev/\sqrt{\frac{N_{t_0} dt}{t_D}} \tag{S26}$$

A typical option for $t_D$ is twice the half-life of the average VACF [3], $t_D = 2\tau$. This is reported in the main text. A more conservative option would be the full length of the VACF window, $t_D \sim 10\tau$. This leads to a factor of 2 uncertainty in the error estimation.


[1] M. Torrent, F. Jollet, F. Bottin, G. Zérah, and X. Gonze, Implementation of the projector augmented-wave method in the ABINIT code: Application to the study of iron under pressure, Computational Materials Science **42**, 337 (2008).

[2] G. Kresse and D. Joubert, From ultrasoft pseudopotentials to the projector augmented-wave method, Phys. Rev. B **59**, 1758 (1999).

[3] E. R. Meyer, J. D. Kress, L. A. Collins, and C. Ticknor, Effect of correlation on viscosity and diffusion in molecular-dynamics simulations, Phys. Rev. E **90**, 043101 (2014).
